# Supplementary material for: Competitions in AI -- Robustly Ranking Solvers Using Statistical Resampling
Source: arXiv:2308.05062 source file (2023-08-09)
Supplement: Supplementary file 2 [file ilsvrc2015_object_detection_additional_data_alt_rankings.tex]

\textbf{Group} & \textbf{Fract. Rank} & \textbf{Solvers} \\
\midrule
     1 & 1    & Amax 2 (1) \\
     2 & 2    & Amax 1 (2) \\
     3 & 3    & CUImage 2 (3) \\
     4 & 4    & MIL-UT 1 (4) \\
     5 & 5    & MIL-UT 2 (5) \\
     6 & 6    & Trimps-Soushen 1 (6) \\
     7 & 7.5    & Trimps-Fudan-HUST 1 (7), Trimps-Soushen 3 (8) \\
     8 & 9    & Futurecrew 2 (9) \\
     9 & 10    & Futurecrew 3 (10) \\
    10 & 11    & Futurecrew 1 (11) \\
    11 & 12    & 1-HKUST 1 (12) \\
    12 & 13    & 1-HKUST 2 (13) \\
