# Supplementary material for: Competitions in AI -- Robustly Ranking Solvers Using Statistical Resampling
Source: arXiv:2308.05062 source file (2023-08-09)
Supplement: Supplementary file 3 [file ilsvrc2015_object_detection_video_additional_data_alt_rankings.tex]

\textbf{Group} & \textbf{Fract. Rank} & \textbf{Solvers} \\
\midrule
     1 & 1.5    & Amax 11 (1), CUVideo 12 (2) \\
     2 & 3.5    & Trimps-Soushen 13 (3), Trimps-Soushen 14 (4) \\
     3 & 5    & BAD 14 (5) \\
     4 & 7    & BAD 12 (6), BAD 13 (7), BAD 11 (8) \\
     5 & 9.5    & BAD 15 (9), NECLAMA 11 (10) \\
