# Supplementary material for: Competitions in AI -- Robustly Ranking Solvers Using Statistical Resampling
Source: arXiv:2308.05062 source file (2023-08-09)
Supplement: Supplementary file 4 [file ilsvrc2015_object_localization_additional_data_alt_rankings.tex]

\textbf{Group} & \textbf{Fract. Rank} & \textbf{Solvers} \\
\midrule
     1 & 1    & Trimps-Soushen 9 (1) \\
     2 & 2    & Amax 6 (2) \\
     3 & 3    & CUImage 7 (3) \\
     4 & 4    & CUImage 8 (4) \\
